# Supplementary material for: Certifiably Robust Policies for Uncertain Parametric Environments
Source: arXiv:2408.03093 source file (2025-03-23)
Supplement: Supplementary file 1 [file experiments.tex]

We present the experiments from Section~\ref{sec:exp} in full detail. Figure~\ref{fig:expfull} shows the results of robust policy learning on different benchmark environments, both with and without model-based optimizations. The full picture shows that model-based optimizations strongly improve the learning speed and the tightness of the obtained guarantee. Additionally, the figure illustrates the parameter distributions underlying the models, which are unknown to the algorithm. For the distributions we either use a uniform distribution or Beta distributions with parameters $\alpha$ and $\beta$ of the form

\begin{equation}
 \text{Beta}(x; \alpha, \beta) = \frac{1}{B(\alpha, \beta)}x^{\alpha-1}(1-x)^{\beta -1},
\end{equation}
where $B(\alpha,\beta) = \frac{(\alpha - 1)! (\beta -1)!}{(\alpha + \beta - 1)!}$ is the beta function.

Figure~\ref{fig:performancediffs} shows the difference of existential, i.e., individual optimal performance on each MDP, compared to the performance of the learned robust policies.

\begin{figure}[htbp]
    \centering

        \begin{subfigure}{\textwidth}
        \centering
        \begin{subfigure}[c]{0.3\textwidth}
            \centering
            \includegraphics[width=\textwidth]{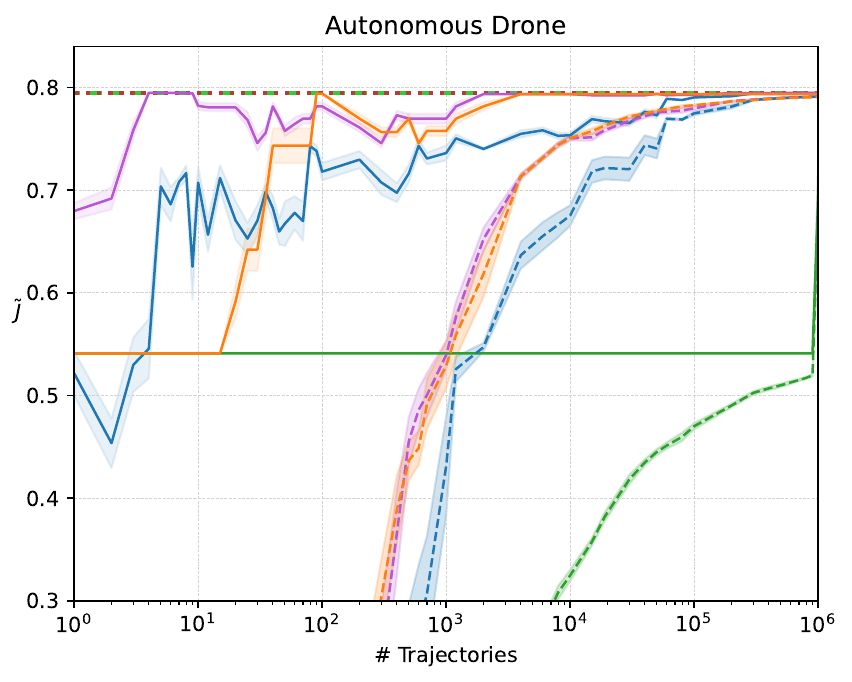}
        \end{subfigure}
        \hfill
        \begin{subfigure}[c]{0.3\textwidth}
            \centering
            \includegraphics[width=\textwidth]{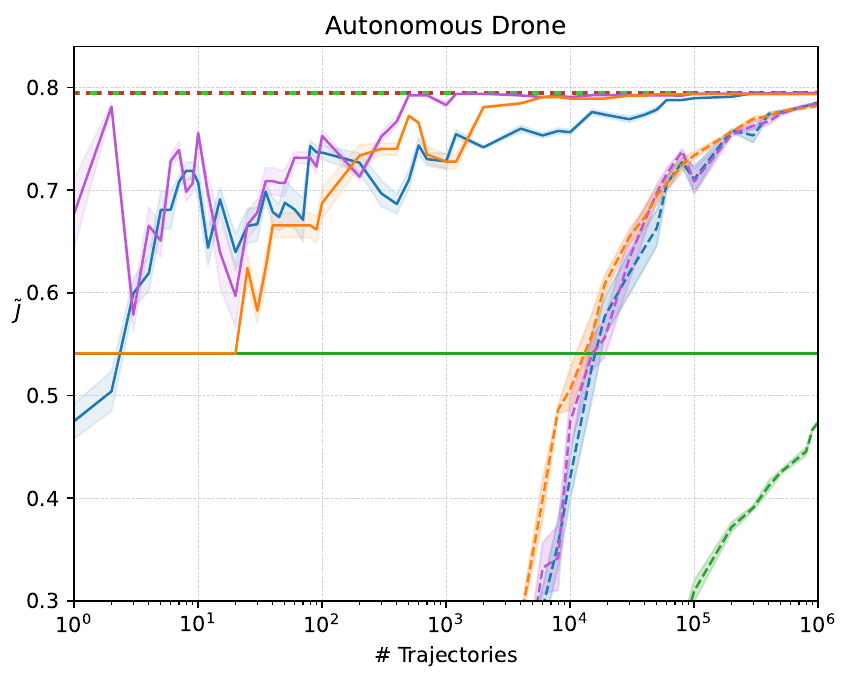}
        \end{subfigure}
        \hfill
        \begin{subfigure}[c]{0.3\textwidth}
            \centering
            \vspace{0.2cm}
            \stackunder{\includegraphics[width=\textwidth]{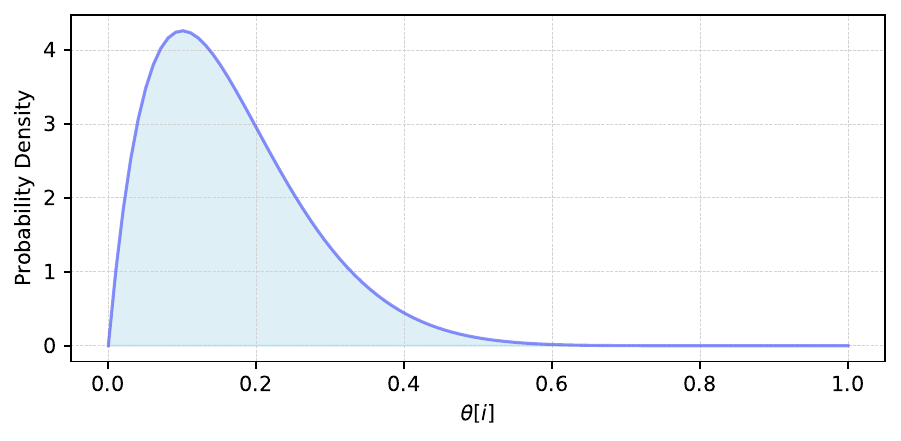}}{{$\quad \mathbb{P}$}}
        \end{subfigure}
        \caption{Autonomous Drone -- $p_i \sim \text{Beta}(2,10)$.}
    \end{subfigure}
    
    \vspace{0.5cm}
    
    % Third row
    \begin{subfigure}{\textwidth}
        \centering
        \begin{subfigure}[c]{0.3\textwidth}
            \centering
            \includegraphics[width=\textwidth]{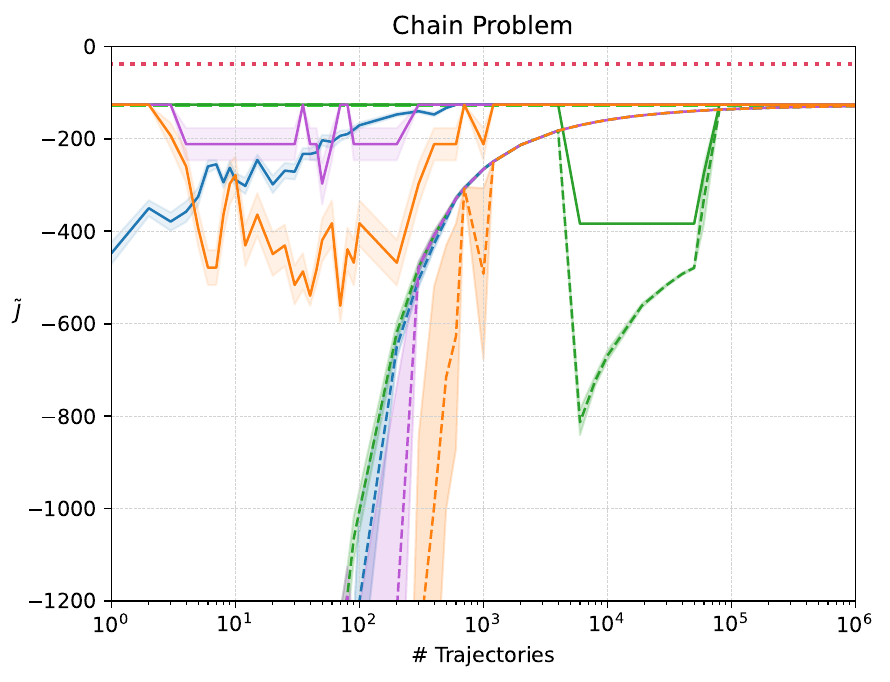}
        \end{subfigure}
        \hfill
        \begin{subfigure}[c]{0.3\textwidth}
            \centering
            \includegraphics[width=\textwidth]{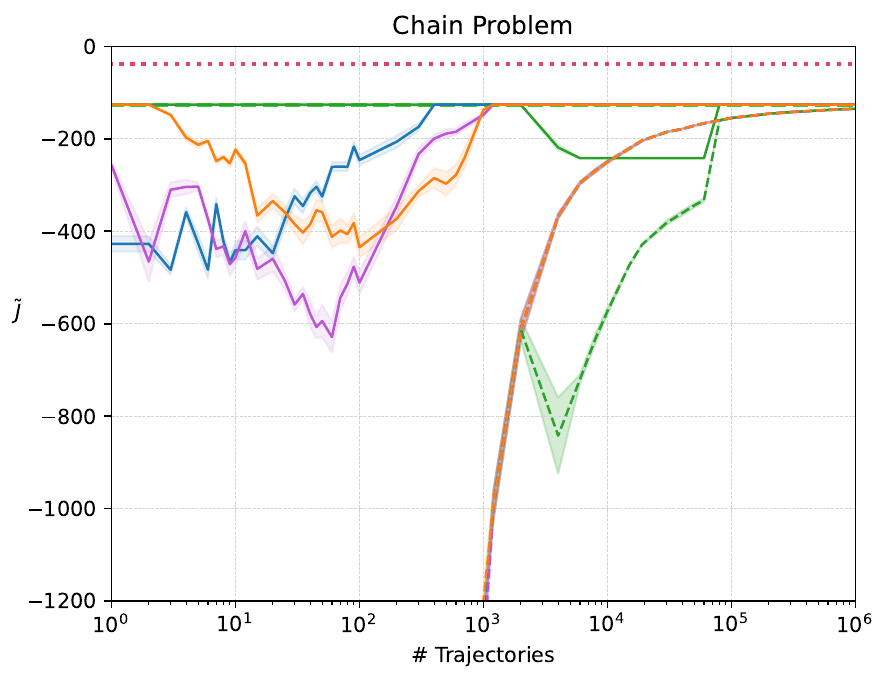}
        \end{subfigure}
        \hfill
        \begin{subfigure}[c]{0.3\textwidth}
            \centering
            \vspace{0.2cm}
            \stackunder{\includegraphics[width=\textwidth]{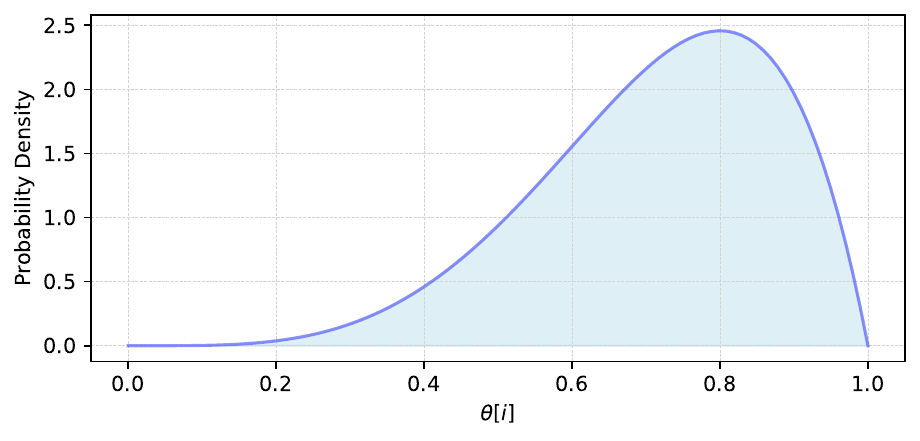}}{$\quad \mathbb{P}$}
        \end{subfigure}
        \caption{Chain Problem -- $p \sim \text{Beta}(5,2)$.}
    \end{subfigure}
    
    \vspace{0.5cm}
    
    % First row
    \begin{subfigure}{\textwidth}
        \centering
        \begin{subfigure}[c]{0.3\textwidth}
            \centering
            \includegraphics[width=\textwidth]{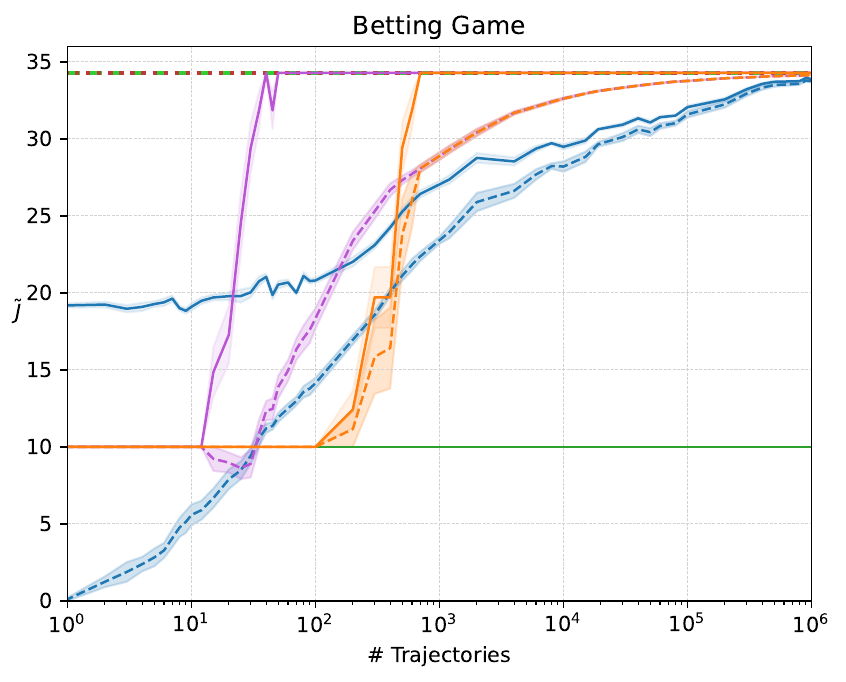}
        \end{subfigure}
        \hfill
        \begin{subfigure}[c]{0.3\textwidth}
            \centering
            \includegraphics[width=\textwidth]{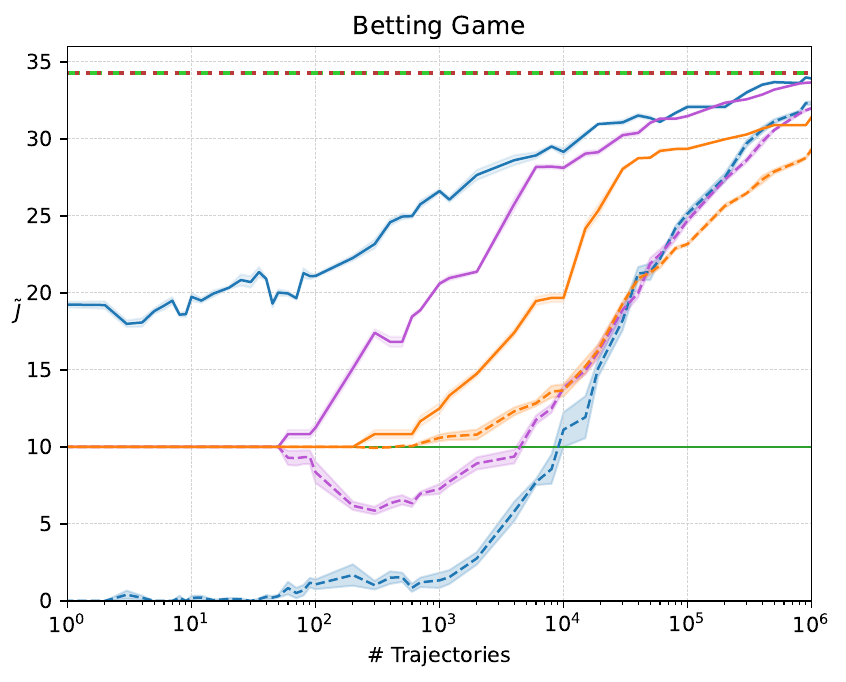}
        \end{subfigure}
        \hfill
        \begin{subfigure}[c]{0.3\textwidth}
            \centering
            \vspace{0.2cm}
            \stackunder{\includegraphics[width=\textwidth]{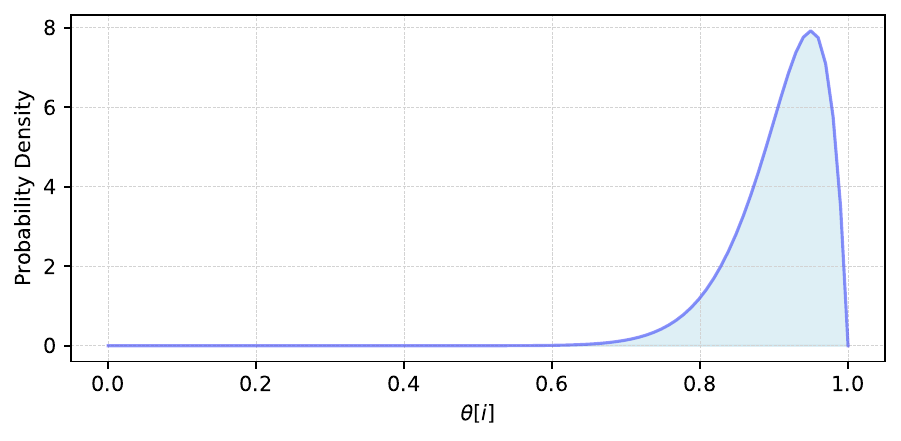}}{$\quad \mathbb{P}$}
            
        \end{subfigure}
        \caption{Betting Game -- $p \sim \text{Beta}(20,2)$.}
    \end{subfigure}
    
    \vspace{0.5cm}
    
    % Second row
    \begin{subfigure}{\textwidth}
        \centering
        \begin{subfigure}[c]{0.3\textwidth}
            \centering
            \includegraphics[width=\textwidth]{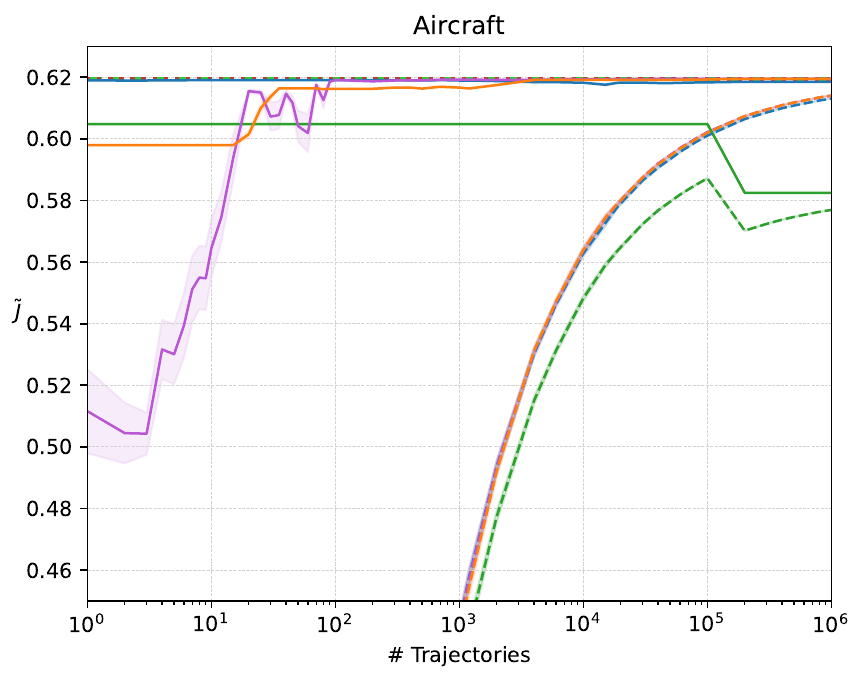}
        \end{subfigure}
        \hfill
        \begin{subfigure}[c]{0.3\textwidth}
            \centering
            \includegraphics[width=\textwidth]{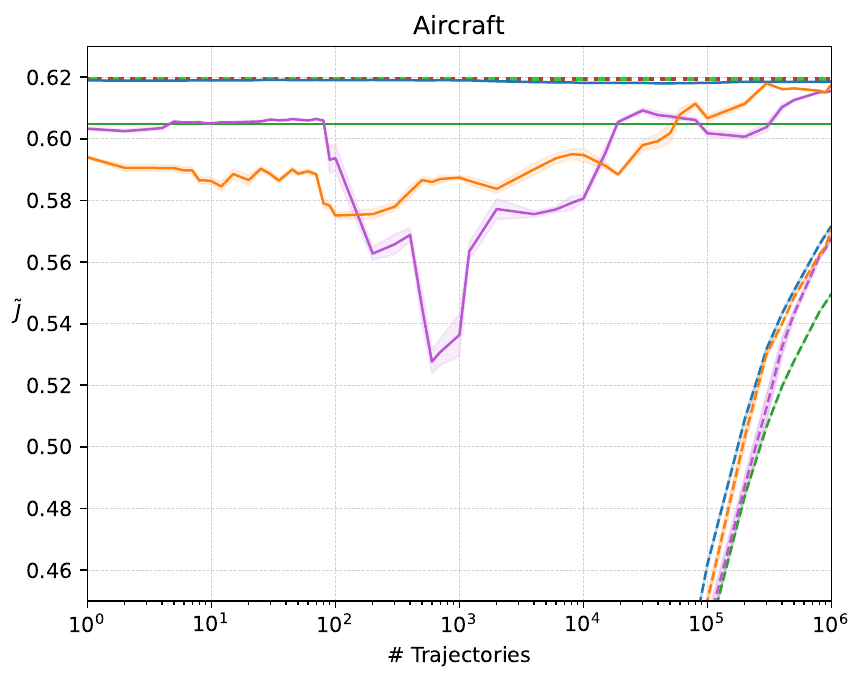}
        \end{subfigure}
        \hfill
        \begin{subfigure}[c]{0.3\textwidth}
            \centering
            \vspace{0.2cm}
            \stackunder{\includegraphics[width=\textwidth]{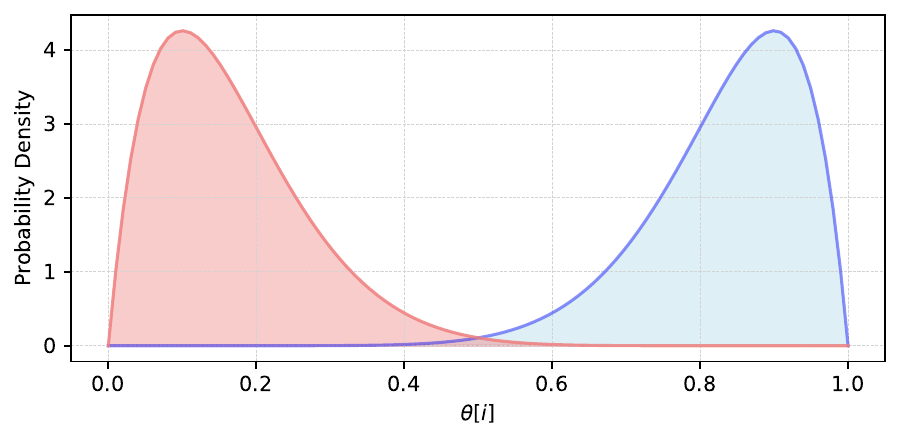}}{{$\quad \mathbb{P}$}}
        \end{subfigure}
        \caption{Aircraft Collision Avoidance -- $p \sim \text{Beta}(10,2)$ and $q \sim \text{Beta}(2,10)$. }
    \end{subfigure}

\vspace{0.5cm}
        % Third row
    \begin{subfigure}{\textwidth}
        \centering
        \begin{subfigure}[c]{0.3\textwidth}
            \centering
            \includegraphics[width=\textwidth]{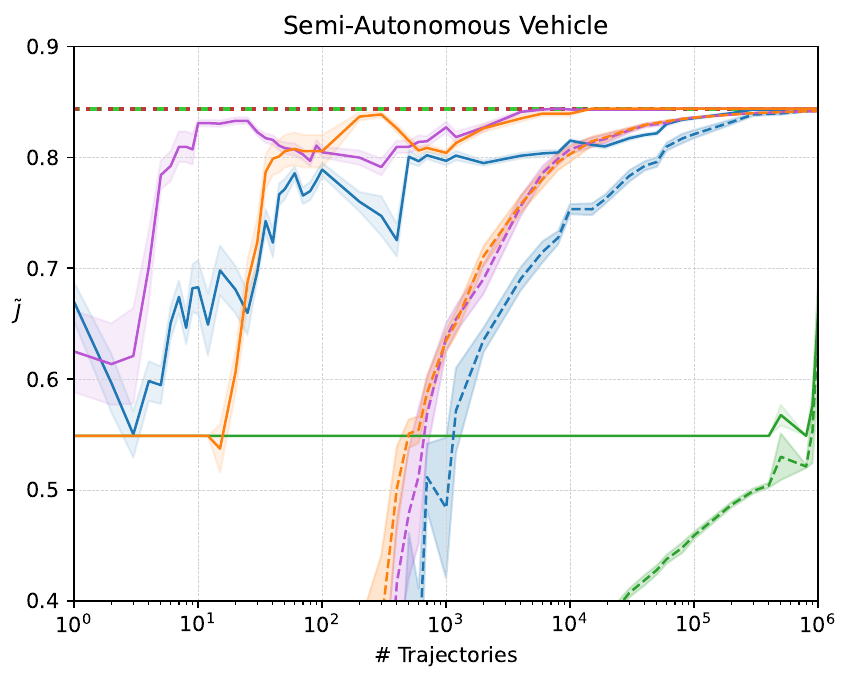}
        \end{subfigure}
        \hfill
        \begin{subfigure}[c]{0.3\textwidth}
            \centering
            \includegraphics[width=\textwidth]{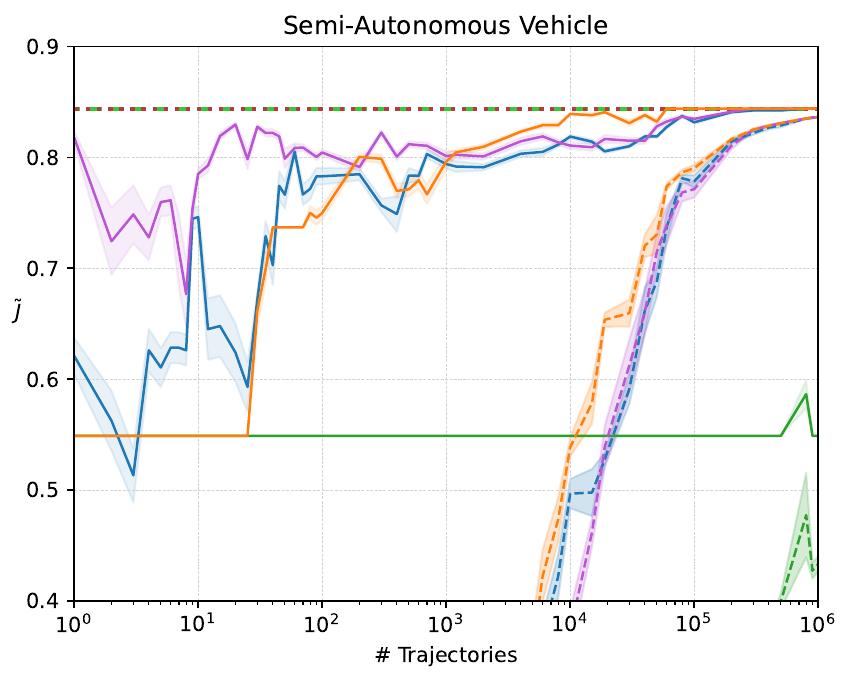}
        \end{subfigure}
        \hfill
        \begin{subfigure}[c]{0.3\textwidth}
            \centering
            \vspace{0.2cm}
            \stackunder{\includegraphics[width=\textwidth]{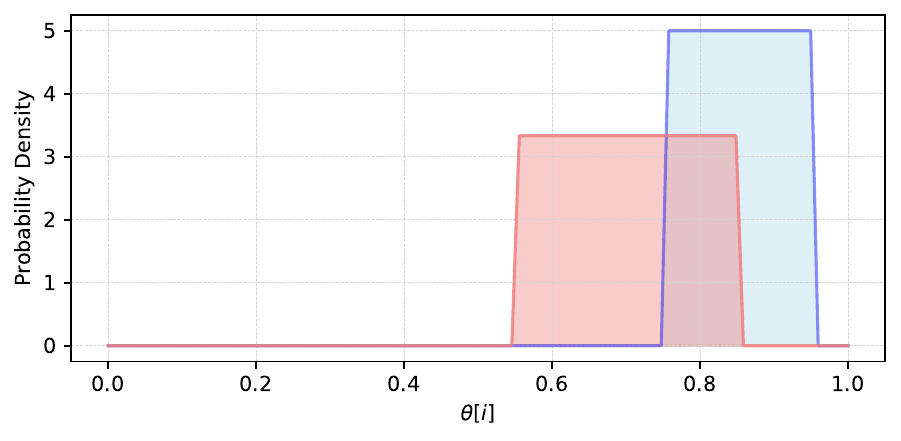}}{$\quad \mathbb{P}$}
        \end{subfigure}
        \caption{Semi-Autonomous Vehicle -- $p \sim \text{Uniform}(0.75,0.95)$ and $q \sim \text{Uniform}(0.55,0.85)$.}
    \end{subfigure}
            % Third row

    \caption{Comparison of robust performances on the unseen verification set and obtained robust performance guarantees using different IMDP learning algorithms, both with model-based optimizations (left column) and without (middle column). The right column illustrates the unknown distribution of the environment parameters.}
    \label{fig:expfull}
    
\end{figure}

\begin{figure}[htbp]
    \centering
    % First subfigure
    \begin{subfigure}{0.45\textwidth}
        \centering
        \includegraphics[width=\textwidth]{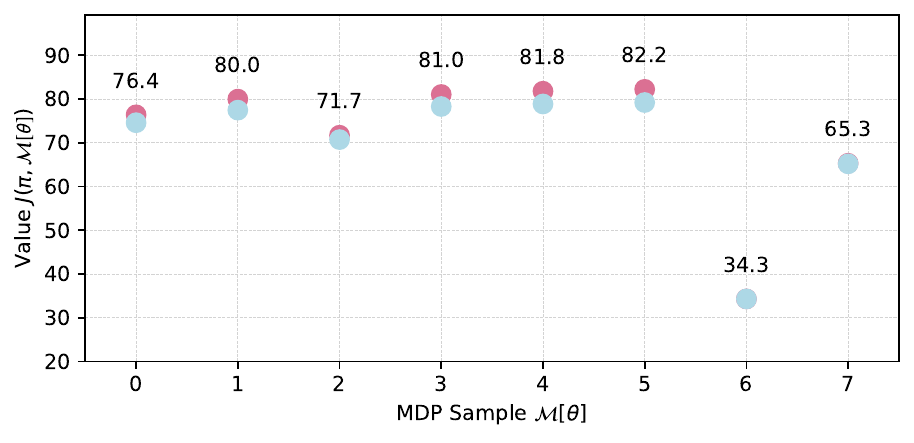}
        \caption{Betting Game.}
    \end{subfigure}
    \hfill
    % Second subfigure
    \begin{subfigure}{0.45\textwidth}
        \centering
        \includegraphics[width=\textwidth]{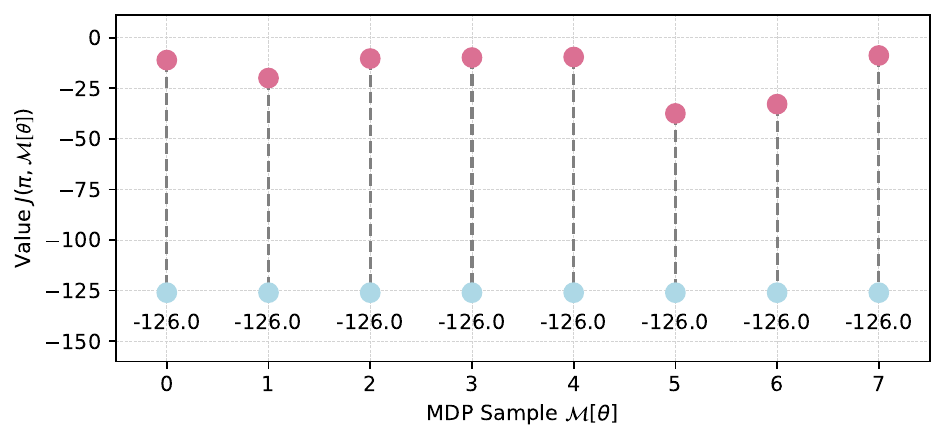}
        \caption{Chain Problem.}
    \end{subfigure}
    \caption{Differences between existential (red dots) and robust performances (blue dots) for a subset of MDP samples. In the betting game, the robust policy is optimal on the worst-case sample and, therefore, not improvable. It is suboptimal on other samples but does not perform worse than on the worst-case sample. For the chain problem, the robust policy is suboptimal on all samples as it chooses the \( \frac{1}{2} \) probability action as the robust middle way.}
    \label{fig:performancediffs}
\end{figure}
