# Supplementary material for: Certifiably Robust Policies for Uncertain Parametric Environments
Source: arXiv:2408.03093 source file (2025-03-23)
Supplement: Supplementary file 2 [file risk_bounds.tex]

We present the risk bounds derived from our main theorems in Section~\ref{sec:riskeval}. Figure~\ref{fig:risknormalfull} displays the risk bounds without discarding any samples, based on Theorem~\ref{thm:bound}, for typical values of IMDP inclusion probability \(1 - \gamma\) and overall confidence \(1 - \eta\). Figure~\ref{fig:riskdiscardfull} illustrates the risk when 5\% of the verification samples are discarded, as determined by Theorem~\ref{thm:bounddiscard}. Figure~\ref{fig:empiricalriskfull} shows the performance of the learned policies on the verification set, along with the performance guarantees \(\tilde{J}\) (without discarding samples) and \(\tilde{J}_k\) (with some samples discarded). We also present the optimal risk bounds \(\varepsilon\) and the actual empirical risk bounds \(\hat{\varepsilon}\), evaluated on an additional 1000 fresh MDP samples.

\begin{figure}[h]
    \centering
    \begin{subfigure}[b]{0.325\textwidth}
        \centering
        \includegraphics[width=\textwidth]{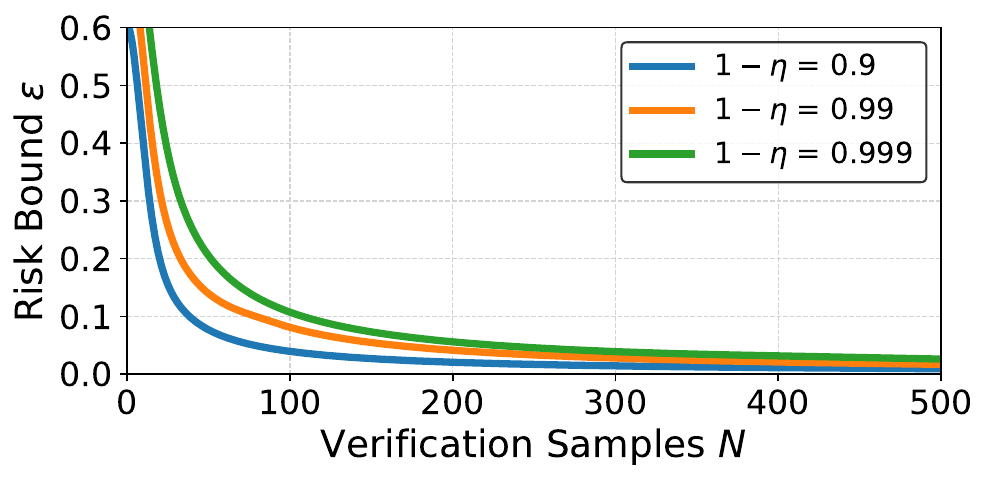}
        \caption{$\gamma = 10^{-4}$}
        \label{fig:subfig1}
    \end{subfigure}
    \hfill
    \begin{subfigure}[b]{0.325\textwidth}
        \centering
        \includegraphics[width=\textwidth]{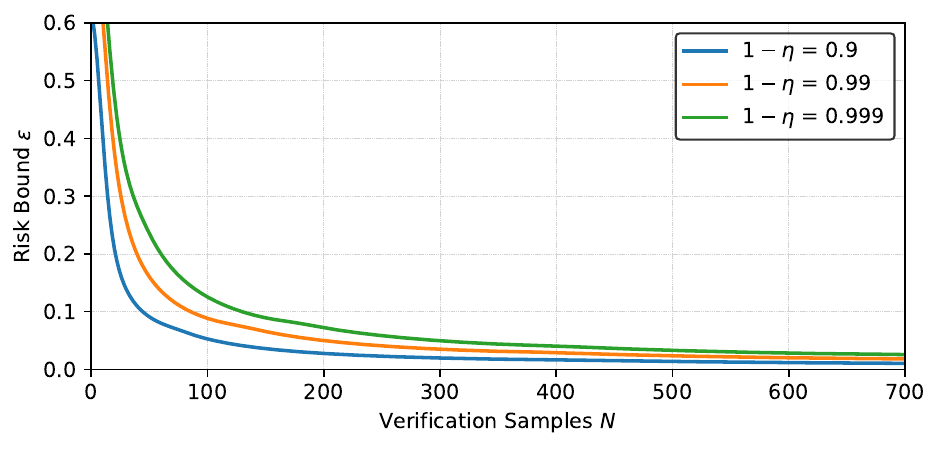}
        \caption{$\gamma = 10^{-3}$}
        \label{fig:subfig2}
    \end{subfigure}
    \hfill
    \begin{subfigure}[b]{0.325\textwidth}
        \centering
        \includegraphics[width=\textwidth]{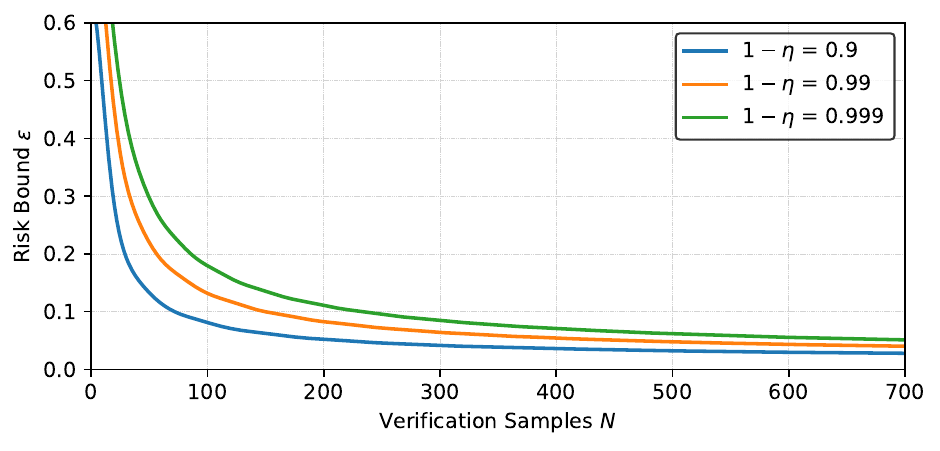}
        \caption{$\gamma = 10^{-2}$}
        \label{fig:subfig3}
    \end{subfigure}
    \caption{Optimal risk bounds as per Theorem~\ref{thm:bound} without discarding of samples.}
    \label{fig:risknormalfull}
\end{figure}

\begin{figure}[h]
    \centering
    \begin{subfigure}[b]{0.325\textwidth}
        \centering
        \includegraphics[width=\textwidth]{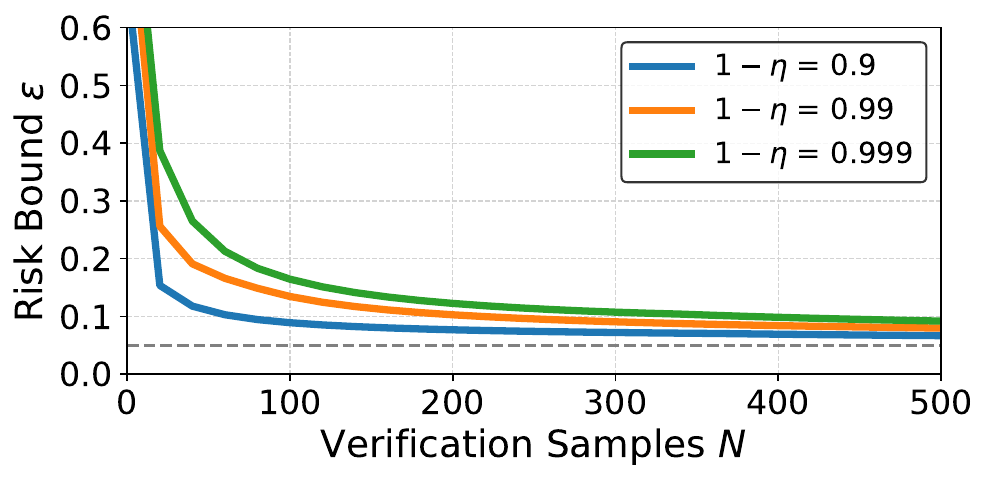}
        \caption{$\gamma = 10^{-4}$}
        \label{fig:subfig1}
    \end{subfigure}
    \hfill
    \begin{subfigure}[b]{0.325\textwidth}
        \centering
        \includegraphics[width=\textwidth]{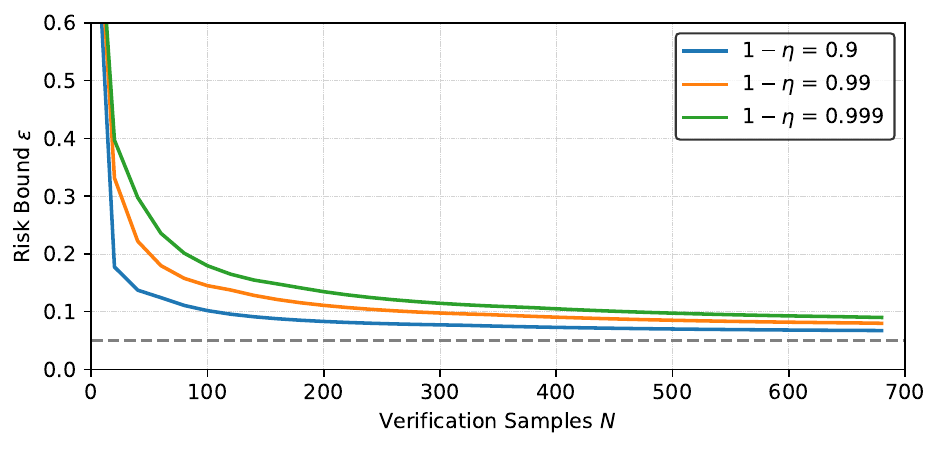}
        \caption{$\gamma = 10^{-3}$}
        \label{fig:subfig2}
    \end{subfigure}
    \hfill
    \begin{subfigure}[b]{0.325\textwidth}
        \centering
        \includegraphics[width=\textwidth]{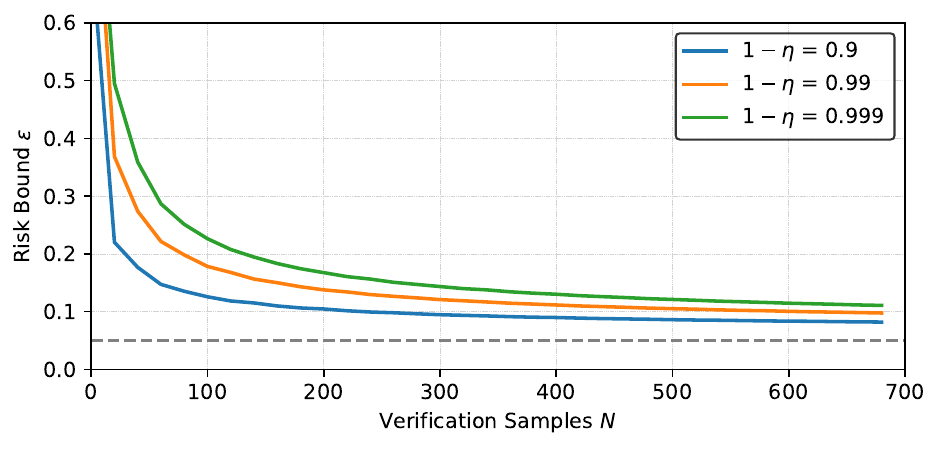}
        \caption{$\gamma = 10^{-2}$}
    \end{subfigure}
    \caption{Optimal risk bounds as per Theorem~\ref{thm:bounddiscard} with discarding $5\%$ of the samples. The bounds are computed for every $N = 20 \cdot k \in \mathbb{N}$. The risk bound approaches the minimum of $0.05$.}
    \label{fig:riskdiscardfull}
\end{figure}

\begin{figure}[h]
    \centering
    \begin{subfigure}[b]{0.325\textwidth}
        \centering
        \includegraphics[width=\textwidth]{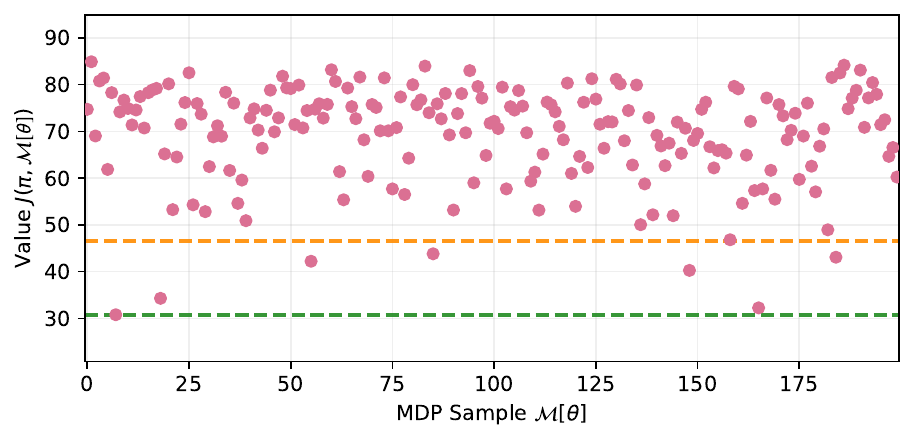}
        \caption{\small Betting Game --$\tilde{J} = 30.4, \varepsilon = 0.04, \hat{\varepsilon} = 0.006,$ and $\tilde{J}_7 = 46.7, \varepsilon_7 = 0.09, \hat{\varepsilon}_7 = 0.04$}
        \label{fig:subfig1}
    \end{subfigure}
    \hfill
    \begin{subfigure}[b]{0.325\textwidth}
        \centering
        \includegraphics[width=\textwidth]{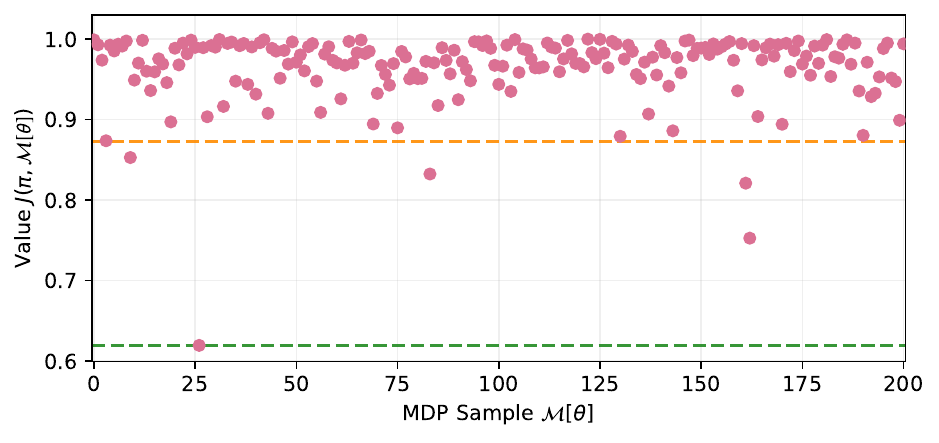}
        \caption{\small Aircraft -- $\tilde{J} = 0.62, \varepsilon = 0.04, \hat{\varepsilon} = 0.002,$ and $\tilde{J}_6 = 0.87, \varepsilon_6 = 0.07, \hat{\varepsilon}_6 = 0.03$}
        \label{fig:subfig2}
    \end{subfigure}
    \hfill
    \begin{subfigure}[b]{0.325\textwidth}
        \centering
        \includegraphics[width=\textwidth]{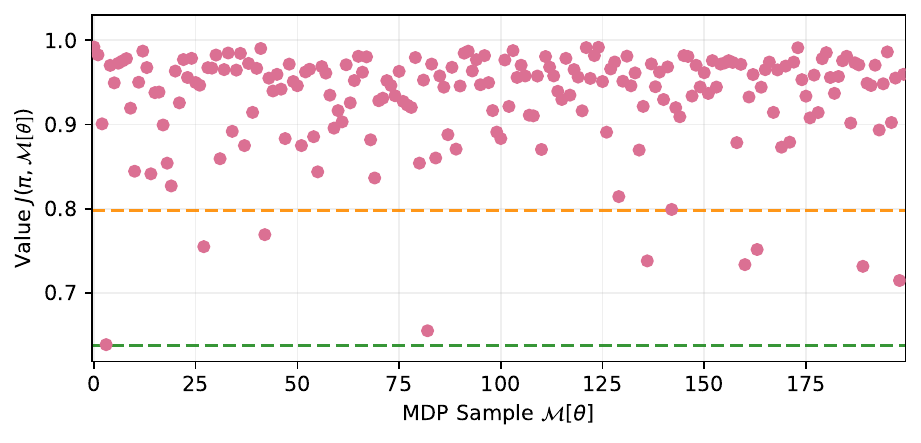}
        \caption{\small Semi Auton.\ Vehicle -- $\tilde{J} = 0.64, \varepsilon = 0.04, \hat{\varepsilon} = 0.004,$ and $\tilde{J}_9 = 0.8, \varepsilon_9 = 0.1, \hat{\varepsilon}_9 = 0.05$}
        \label{fig:subfig3}
    \end{subfigure}
    \caption{Performance of the learned policies on a verification set together with computed risk bounds $\varepsilon$. empirical risk $\hat{\varepsilon}$ and sample discarding bounds.}
    \label{fig:empiricalriskfull}
\end{figure}
